# Supplementary material for: Multimodal Large Language Models as Image Classifiers
Source: arXiv:2603.06578 source file (2026-10-08)
Supplement: Supplementary file 1 [file chatgpt-n-group.tex]

\begin{table*}[h]
\small
\centering
\begin{tabular}{lcccccccccccc}
\toprule
Batch & Is Shuffled & $\mathrm{Acc}_{gt}^{1360}$ & N/A \\
\cmidrule{1-4}
10 & True & 47.79 & 303 \\
\bottomrule
\end{tabular}
\vspace{1em}
\caption{N group evaluation.}
\label{tab:n_group}
\end{table*}
